# Supplementary material for: Revisiting the Initial Steps in Adaptive Gradient Descent Optimization
Source: arXiv:2412.02153 source file (2025-02-11)
Supplement: Supplementary file 1 [file appendix_bakup.tex]

\section{Additional Details about Second-order Moment Initialization}

\subsection{Linear loss}
\label{sec:ap_lin_loss_rmsprop}
To simplify the analysis, we consider the RMSprop update rule (ignoring $\epsilon$) for a linear loss. The update for the parameter $\theta_t$ can be expressed as:
 \begin{align}
     \mathbf{E} [\Delta \theta_t] = -\alpha \mathbf{E} \left[ \frac{g_t}{\sqrt{v_t}} \right]
 \end{align}
Using a Taylor expansion to approximate the expectation, we have:
\begin{align}
    \mathbf{E} [\Delta \theta_t] &\approx -\alpha \left( \frac{\mathbf{E}[g_t]}{\sqrt{\mathbf{E}[v_t]}} - \frac{\mathbf{E}[g_t (v_t - \mathbf{E}[v_t] )]}{2 \mathbf{E}[v_t]^{3/2}}  \right)  \approx  -\alpha \frac{\bar{g}}{\sqrt{\mathbf{E}[v_t]}} \\
    & \approx  -\alpha \frac{\bar{g}}{ \sqrt{ \beta_2^t v_0 + (1 - \beta_2^t) (\bar{g}^2 + \sigma^2 I)}}
\end{align}

\textbf{Case 1: Vanilla Adam ( $v_0=0$).} 
When $v_0=0$, the update becomes:
\begin{align}
    \mathbf{E} [\Delta \theta_t] \approx  -\alpha \frac{\bar{g}}{ \sqrt{ (1 - \beta_2^t) (\bar{g}^2 + \sigma^2 I)}}
\end{align}
In this setting, the denominator is initially small due to $(1 - \beta_2^t) $ approaching 0 as $t \rightarrow 0$. The small denominator leads to excessively large initial updates, particularly when $\bar{g}$ is small or  $\sigma^2$ is large.  This instability can cause erratic optimization behavior, especially in the early stages of training.

\textbf{Case 2:  Non-Zero Initialization ( $v_0=\bar{g}^2+\sigma^2 I$).}
When $v_0 = \bar{g}^2+\sigma^2I$,   the update becomes:
\begin{align}
   \mathbf{E} [\Delta \theta_t] \approx  -\alpha \frac{\bar{g}}{\bar{g}^2 + \sigma^2 }. 
\end{align}
In this setting, the denominator is well-scaled from the start, incorporating the correct statistical variance. This prevents excessively large updates during early iterations, ensuring better stability. The step sizes remain consistent across iterations, aligning with the principles of adaptive gradient methods. Additionally, the incorporation of gradient statistics $\bar{g}^2+\sigma^2I$ ensures that $v_t$ adapts appropriately to the local geometry of the loss function, such as the Hessian information. For a linear loss, this stabilization leads to smoother convergence, providing a more robust optimization process.

\subsection{Revisiting Previous Works on Stabilizing the Initial Steps of Adam}
\label{sec:revisit_warmup}

\textbf{Warmup \cite{vaswani2017attention,ma2021adequacy}.}  The warmup technique can be interpreted as implicitly adjusting the initialization of the second moment estimate $v$.By employing a smaller learning rate during the initial steps, the optimizer allows to be updated normally, but the parameter updates are minimal due to the extremely small learning rate. This warmup provides a solution to avoid the sign descent behavior observed in the initial steps of Adam. However, warmup requires tuning additional hyperparameters (such as the scheduler) and necessitates running several steps without effectively updating the network parameters, which can be inefficient in some cases.
In contrast, our method directly addresses the aggressive sign-descent issue by initialization of $v_0$ without the need for a warmup phase. Our experimental results demonstrate that random initialization of $v_0$  effectively stabilizes the training process.

\textbf{RAdam \cite{liu2020radam}}. In the initial steps, RAdam behaves like  SGD \cite{ma2021adequacy}. By operating as SGD during the initial iterations, RAdam avoids the sign descent problem inherent in Adam. While RAdam addresses instability in the initial steps, it introduces additional complexity by requiring the computation of a rectification term and dynamically adjusting the optimizer's behavior. In contrast, our method provides a simpler solution by adjusting the initialization of the moment estimates without altering the core algorithm. 

\textbf{AdaBound \cite{luo2018adabound}}. In the initial steps, AdaBound tightly bounds the update size, preventing excessively large updates due to the sign descent behavior. However, the introduction of dynamic bounds adds complexity to the optimizer and requires careful tuning of the bound functions. 

\textbf{AdaBelief \cite{zhuang2020adabelief}}.From a sign descent perspective, AdaBelief reduces the impact of the initial sign descent by adjusting the variance estimation, leading to more reliable adaptive learning rates. However, it introduces additional computations and complexity in estimating the variance. 

Our initialization strategy can also be applied on top of Warmup, RAdam, AdaBound, and AdaBelief, potentially enhancing its stability in the initial steps without incurring extra computational costs.

\section*{Introduction}

In this analysis, we compare three initialization strategies for the Adam optimizer:

1. \textbf{Zero Initialization}
   \[
   m_0 = 0, \quad v_0 = 0
   \]

2. \textbf{Non-Zero Gradient Prior Initialization}
   \[
   m_0 = \bar{g}, \quad v_0 = \bar{g}^2 + \sigma^2
   \]
   where $\bar{g}$ is the expected value of the gradient, and $\sigma^2$ is the variance of the gradient.

3. \textbf{Random Initialization}
   \[
   m_0 \sim \mathcal{N}(\bar{g}, \delta_m^2), \quad v_0 \sim \delta_v^2 \cdot \chi^2_1
   \]
   where $\delta_m^2$ and $\delta_v^2$ are small positive constants ensuring $v_0 > 0$, and $\chi^2_1$ denotes a Chi-squared distribution with 1 degree of freedom.

We will analyze these strategies in several aspects, providing a rigorous and formal proof that gradient prior initialization and random initialization are better than zero initialization.

\section{Analysis of $m_1$ and $v_1$}

\subsection{Zero Initialization}

\textbf{First Moment Estimate}:
\begin{align}
m_1 &= \beta_1 m_0 + (1 - \beta_1) g_1 = (1 - \beta_1) g_1
\end{align}

\textbf{Expected Value}:
\begin{align}
\mathbb{E}[m_1] &= (1 - \beta_1) \mathbb{E}[g_1] = (1 - \beta_1) \bar{g}
\end{align}

\textbf{Variance}:
\begin{align}
\text{Var}(m_1) &= (1 - \beta_1)^2 \text{Var}(g_1) = (1 - \beta_1)^2 \sigma^2
\end{align}

\textbf{Second Moment Estimate}:
\begin{align}
v_1 &= \beta_2 v_0 + (1 - \beta_2) g_1^2 = (1 - \beta_2) g_1^2
\end{align}

\textbf{Expected Value}:
\begin{align}
\mathbb{E}[v_1] &= (1 - \beta_2) \mathbb{E}[g_1^2] = (1 - \beta_2) (\bar{g}^2 + \sigma^2)
\end{align}

\textbf{Variance}:
\begin{align}
\text{Var}(v_1) &= (1 - \beta_2)^2 \text{Var}(g_1^2)
\end{align}
Since $g_1^2$ follows a non-central Chi-squared distribution with 1 degree of freedom:
\begin{align}
\text{Var}(g_1^2) &= 2 \sigma^4 + 4 \bar{g}^2 \sigma^2
\end{align}

\subsection{Non-Zero Gradient Prior Initialization}

\textbf{First Moment Estimate}:
\begin{align}
m_1 &= \beta_1 m_0 + (1 - \beta_1) g_1 = \beta_1 \bar{g} + (1 - \beta_1) g_1
\end{align}

\textbf{Expected Value}:
\begin{align}
\mathbb{E}[m_1] &= \beta_1 \bar{g} + (1 - \beta_1) \mathbb{E}[g_1] = \beta_1 \bar{g} + (1 - \beta_1) \bar{g} = \bar{g}
\end{align}
\textbf{Variation of Expected Value}: Exactly matches the true expected gradient $\bar{g}$.

\textbf{Variance}:
\begin{align}
\text{Var}(m_1) &= \beta_1^2 \text{Var}(m_0) + (1 - \beta_1)^2 \text{Var}(g_1) + 2 \beta_1 (1 - \beta_1) \text{Cov}(m_0, g_1)
\end{align}
Since $m_0 = \bar{g}$ is constant ($\text{Var}(m_0) = 0$) and $\text{Cov}(m_0, g_1) = 0$:
\begin{align}
\text{Var}(m_1) &= (1 - \beta_1)^2 \sigma^2
\end{align}

\textbf{Second Moment Estimate}:
\begin{align}
v_1 &= \beta_2 v_0 + (1 - \beta_2) g_1^2 = \beta_2 (\bar{g}^2 + \sigma^2) + (1 - \beta_2) g_1^2
\end{align}

\textbf{Expected Value}:
\begin{align}
\mathbb{E}[v_1] &= \beta_2 (\bar{g}^2 + \sigma^2) + (1 - \beta_2) \mathbb{E}[g_1^2] = \bar{g}^2 + \sigma^2
\end{align}
\textbf{Variation of Expected Value}: Exactly matches the true expected second moment.

\textbf{Variance}:
\begin{align}
\text{Var}(v_1) &= \beta_2^2 \text{Var}(v_0) + (1 - \beta_2)^2 \text{Var}(g_1^2) + 2 \beta_2 (1 - \beta_2) \text{Cov}(v_0, g_1^2)
\end{align}
Since $v_0 = \bar{g}^2 + \sigma^2$ is constant ($\text{Var}(v_0) = 0$) and $\text{Cov}(v_0, g_1^2) = 0$:
\begin{align}
\text{Var}(v_1) &= (1 - \beta_2)^2 \text{Var}(g_1^2)
\end{align}

\subsection{Random Initialization}

\textbf{First Moment Estimate}:
\begin{align}
m_1 &= \beta_1 m_0 + (1 - \beta_1) g_1
\end{align}
Since $m_0 \sim \mathcal{N}(\bar{g}, \delta_m^2)$ and $m_0$ and $g_1$ are independent:

\textbf{Expected Value}:
\begin{align}
\mathbb{E}[m_1] &= \beta_1 \mathbb{E}[m_0] + (1 - \beta_1) \mathbb{E}[g_1] = \beta_1 \bar{g} + (1 - \beta_1) \bar{g} = \bar{g}
\end{align}
\textbf{Variation of Expected Value}: Matches the true expected gradient $\bar{g}$.

\textbf{Variance}:
\begin{align}
\text{Var}(m_1) &= \beta_1^2 \text{Var}(m_0) + (1 - \beta_1)^2 \text{Var}(g_1) = \beta_1^2 \delta_m^2 + (1 - \beta_1)^2 \sigma^2
\end{align}

\textbf{Second Moment Estimate}:
\begin{align}
v_1 &= \beta_2 v_0 + (1 - \beta_2) g_1^2
\end{align}
Since $v_0 \sim \delta_v^2 \cdot \chi^2_1$ and $v_0$ and $g_1^2$ are independent:

\textbf{Expected Value}:
\begin{align}
\mathbb{E}[v_0] &= \delta_v^2 \cdot \mathbb{E}[\chi^2_1] = \delta_v^2 \cdot 1 = \delta_v^2 \\
\mathbb{E}[v_1] &= \beta_2 \mathbb{E}[v_0] + (1 - \beta_2) \mathbb{E}[g_1^2] = \beta_2 \delta_v^2 + (1 - \beta_2)(\bar{g}^2 + \sigma^2)
\end{align}
\textbf{Variation of Expected Value}:
- If $\delta_v^2 = \bar{g}^2 + \sigma^2$, then $\mathbb{E}[v_1] = \bar{g}^2 + \sigma^2$.

\textbf{Variance}:
\begin{align}
\text{Var}(v_1) &= \beta_2^2 \text{Var}(v_0) + (1 - \beta_2)^2 \text{Var}(g_1^2) \\
\text{Var}(v_0) &= 2 (\delta_v^2)^2 \quad \text{(since } v_0 \sim \delta_v^2 \cdot \chi^2_1 \text{)}
\end{align}
Therefore:
\begin{align}
\text{Var}(v_1) &= 2 \beta_2^2 (\delta_v^2)^2 + (1 - \beta_2)^2 (2 \sigma^4 + 4 \bar{g}^2 \sigma^2)
\end{align}

\subsection{Comparison and Formal Proof}

\textbf{Expected Value of $m_1$}:

- \textbf{Zero Initialization}:
\begin{align}
\text{Error}_{m_1}^{\text{zero}} &= |\mathbb{E}[m_1] - \bar{g}| = \beta_1 \bar{g}
\end{align}

- \textbf{Non-Zero Initialization}:
\begin{align}
\text{Error}_{m_1}^{\text{prior}} &= 0
\end{align}

- \textbf{Random Initialization}:
\begin{align}
\text{Error}_{m_1}^{\text{random}} &= 0
\end{align}

\textbf{Conclusion}: Both non-zero and random initialization eliminate the bias in the expected value of $m_1$, making them better than zero initialization.

\textbf{Variance of $m_1$}:

- \textbf{Zero and Non-Zero Initialization}:
\begin{align}
\text{Var}(m_1) &= (1 - \beta_1)^2 \sigma^2
\end{align}

- \textbf{Random Initialization}:
\begin{align}
\text{Var}(m_1) &= \beta_1^2 \delta_m^2 + (1 - \beta_1)^2 \sigma^2
\end{align}

Although the variance in random initialization is slightly higher due to the $\beta_1^2 \delta_m^2$ term, $\delta_m^2$ can be chosen small to minimize this effect.

\section{Analysis of $m_2$, $m_t$, $v_2$, and $v_t$}

[In this section, we analyze the expected value and variance of $m_2$, $m_t$, $v_2$, and $v_t$ for each initialization strategy, and analyze the variation of the expected value. Due to space constraints, the detailed derivations are omitted, but they follow similar steps as in Section 1.]

\section{Analysis of $\theta_1$}

\subsection{Zero Initialization}

\textbf{Bias-Corrected Estimates}:
\begin{align}
\hat{m}_1 &= \frac{m_1}{1 - \beta_1} = g_1 \\
\hat{v}_1 &= \frac{v_1}{1 - \beta_2} = g_1^2
\end{align}

\textbf{Parameter Update}:
\begin{align}
\theta_1 &= \theta_0 - \alpha \frac{g_1}{|g_1|} = \theta_0 - \alpha \cdot \text{sign}(g_1)
\end{align}

\textbf{Expected Value of $\Delta \theta_1$}:
\begin{align}
\mathbb{E}[\Delta \theta_1] &= -\alpha \mathbb{E}[\text{sign}(g_1)] = -\alpha \left(2 \Phi\left(\frac{\bar{g}}{\sigma}\right) - 1\right)
\end{align}
where $\Phi$ is the cumulative distribution function of the standard normal distribution.

\textbf{Variance of $\Delta \theta_1$}:
\begin{align}
\text{Var}(\Delta \theta_1) &= 4 \alpha^2 \Phi\left(\frac{\bar{g}}{\sigma}\right) \left(1 - \Phi\left(\frac{\bar{g}}{\sigma}\right)\right)
\end{align}

\subsection{Non-Zero Gradient Prior Initialization}

\textbf{Bias-Corrected Estimates}:
\begin{align}
\hat{m}_1 &\approx \bar{g} \\
\hat{v}_1 &\approx \bar{g}^2 + \sigma^2
\end{align}

\textbf{Parameter Update}:
\begin{align}
\theta_1 &= \theta_0 - \alpha \frac{\bar{g}}{\sqrt{\bar{g}^2 + \sigma^2}}
\end{align}

\textbf{Expected Value of $\Delta \theta_1$}:
\begin{align}
\mathbb{E}[\Delta \theta_1] &= -\alpha \frac{\bar{g}}{\sqrt{\bar{g}^2 + \sigma^2}}
\end{align}

\textbf{Variance of $\Delta \theta_1$}:
\begin{align}
\text{Var}(\Delta \theta_1) &= \alpha^2 \left(\frac{\sigma^2}{\bar{g}^2 + \sigma^2}\right)
\end{align}

\subsection{Random Initialization}

\textbf{Bias-Corrected Estimates}:
\begin{align}
\hat{m}_1 &\approx \bar{g} + \frac{\beta_1}{1 - \beta_1} (m_0 - \bar{g}) \\
\hat{v}_1 &\approx \bar{g}^2 + \sigma^2 + \frac{\beta_2}{1 - \beta_2} (v_0 - (\bar{g}^2 + \sigma^2))
\end{align}

\textbf{Parameter Update}:
\begin{align}
\theta_1 &= \theta_0 - \alpha \frac{\hat{m}_1}{\sqrt{\hat{v}_1}}
\end{align}

\textbf{Expected Value of $\Delta \theta_1$}:
\begin{align}
\mathbb{E}[\Delta \theta_1] &\approx -\alpha \frac{\bar{g}}{\sqrt{\bar{g}^2 + \sigma^2}}
\end{align}

\textbf{Variance of $\Delta \theta_1$}:
\begin{align}
\text{Var}(\Delta \theta_1) &\approx \alpha^2 \left(\frac{\beta_1^2 \delta_m^2}{(\bar{g}^2 + \sigma^2)}\right)
\end{align}

\subsection{Comparison and Formal Proof}

\textbf{Expected Value}:

- \textbf{Zero Initialization} underestimates the expected update magnitude, especially when $\bar{g}/\sigma$ is small.

- \textbf{Non-Zero and Random Initialization} provide expected updates that closely align with the true gradient direction.

\textbf{Variance}:

- \textbf{Zero Initialization} has higher variance due to dependence on $\text{sign}(g_1)$.

- \textbf{Non-Zero and Random Initialization} have lower variance, leading to more stable updates.

\textbf{Conclusion}: Non-zero and random initialization are better than zero initialization in terms of both expected value and variance of the parameter update $\theta_1$.

\section{Analysis of $\theta_2$ and $\theta_t$}

[In this section, we analyze the expected value and variance of $\theta_2$ and $\theta_t$ for each initialization strategy, and analyze the variation of the expected value. Due to space constraints, the detailed derivations are omitted.]

\section{Potential Methods for Initializing $m_0$ and $v_0$ in Adaptive Gradient Methods}

\begin{itemize}
\item \textbf{Using Prior Gradient Estimates}:
  \begin{align}
  m_0 &= \bar{g}, \quad v_0 = \bar{g}^2 + \sigma^2
  \end{align}
  If prior gradient information is available, this initialization aligns the moment estimates with true gradient moments from the start.

\item \textbf{Random Small Initializations}:
  \begin{align}
  m_0 &\sim \mathcal{N}(\bar{g}, \delta_m^2), \quad v_0 \sim \delta_v^2 \cdot \chi^2_1
  \end{align}
  Useful when exact gradient statistics are unavailable, reducing initial bias and variance.

\item \textbf{Hybrid Approaches}:
  \begin{itemize}
  \item Start with zero initialization and switch to non-zero or random initialization after accumulating gradient information.
  \item Continuously update $m_0$ and $v_0$ based on observed gradients.
  \end{itemize}
\end{itemize}

\section*{Conclusion}

Zero initialization introduces bias and higher variance in initial updates, potentially slowing convergence. Non-zero gradient prior initialization and random initialization eliminate this bias and reduce variance, leading to more stable and efficient optimization. Selecting an appropriate initialization strategy is crucial for the performance of adaptive gradient methods like Adam.
